# Supplementary material for: Metastability of lipid necks via geometric triality
Source: arXiv:2101.01161 ancillary file (2021-01-04)
Supplement: Supplementary file 1 [file SI.pdf]

# Supporting Information for: Metastability of lipid necks via geometric triality

Piermarco Fonda[1, 2, *] and Luca Giomi[2]

[1] *Theory & Bio-Systems, Max Planck Institute of Colloids and Interfaces, Am Mühlenberg 1, 14476 Potsdam*
[2] *Instituut-Lorentz, Universiteit Leiden, P.O. Box 9506, 2300 RA Leiden, Netherlands*

[*] piermarco.fonda@mpikg.mpg.de

**CONTENTS**

I. Notation, definitions and general facts 2
I.1. Shape equation 4
I.2. Stresses and the Darboux frame 4
I.3. The boundary conditions for adhesion 5
I.4. Special conformal transformations 6
I.5. Weyl transformations 7
I.6. Maximally symmetric spaces 8
I.7. Axisymmetric surfaces 8
I.7.1. Arc-length parametrization 9
I.7.2. Isothermal parametrization 9

II. Proof of Eq. 2 10
II.1. A simple check 11

III. Proof of Eq. 3 11
III.1. Elastica equilibrium equation 12

IV. Construction of the hyperbolic neck solution, Eq. 4 12
IV.1. Analytic expression of geometric quantities 15
IV.2. The adhesion equation 16

References 16

## I. NOTATION, DEFINITIONS AND GENERAL FACTS

We consider a surface $S$ embedded in a three-dimensional manifold $M_3$. This embedding is defined by a map

$$\sigma^i \mapsto r^\mu(\sigma^i)\,, \tag{S1.1}$$

from (a subset of) $\mathbb{R}^2$ - parametrized by the two generic coordinates $\sigma^1$ and $\sigma^2$ - to $M_3$.

In the following, Latin indices $i, j, k, \ldots$ refer to components of tensors on $S$, Greek indices $\mu, \nu, \rho, \ldots$ refer to components of tensors on $M_3$. Round and square brackets on indices imply respectively symmetric and antisymmetric parts of tensors. We suppose $S$ to be orientable and not self-intersecting.

We further suppose that $M_3$ is equipped with a positive-defined metric $g_{\mu\nu}$, with inverse $g^{\mu\nu}$. When $M_3 = \mathbb{R}^3$, this becomes the identity matrix $g_{\mu\nu} = \delta_{\mu\nu}$. In this case, we replace the Greek indices notation with bold characters, i.e. we write $\boldsymbol{r}$ for $r^\mu$.

The components of the tangent vectors on $S$ are defined as

$$t^\mu_i = \partial_i r^\mu\,, \tag{S1.2}$$

where $\partial_i$ is the ordinary derivative with respect to $\sigma^i$. From this we can construct the *induced metric*

$$h_{ij} = g_{\mu\nu} t^\mu_i t^\nu_j\,, \tag{S1.3}$$

which is a symmetric tensor and admits inverse $h^{ij}$. We can use $h_{ij}$ and $g_{\mu\nu}$ and their inverses to raise and lower indexes in the respective tangent spaces.

Since this embedding has codimension one, we can construct explicitly the normal vector field over $S$ using Levi-Civita symbols:

$$n_\mu = \frac{1}{\sqrt{\det h}} \epsilon^{ij} \epsilon_{\mu\nu\rho} t^\nu_i t^\rho_j\,, \tag{S1.4}$$

where $\det h$ is the determinant of the induced metric, Eq. (S1.3), and $\epsilon^{12} = \epsilon_{123} = 1$. This vector field has the desirable properties of $n_\mu t^\mu_i = 0$ and $n_\mu n_\nu g^{\mu\nu} = 1$.

With the help of Eq. (S1.3) we can decompose the ambient metric as

$$g_{\mu\nu} = t_{i\mu} t_{j\nu} h^{ij} + n_\mu n_\nu\,. \tag{S1.5}$$

From either $g$ or $h$ it is possible to construct Levi-Civita connections, so to define metric-compatible covariant derivatives $\nabla_\mu$ (on $TM_3$) and $\nabla_i$ (on $TS$).

With the covariant derivative on $M_3$ and the frame decomposition into normal and tangential components one gets one of the Gauss-Weingarten relations

$$t_i^\mu \nabla_\mu n^\nu = K_{ij} t^{\mu j}\,, \tag{S1.6}$$

which allows us to introduce the symmetric *extrinsic curvature tensor*

$$K_{ij} = t_i^\mu t_j^\nu \nabla_\mu n_\nu\,. \tag{S1.7}$$

Furthermore, from $h$ and its Levi-Civita connection we can construct the two-dimensional Riemann tensors $\mathcal{R}_{ijkl}$. Similarly, we construct the three-dimensional Riemann tensor $R_{\mu\nu\rho\sigma}$ from $g_{\mu\nu}$.

It is useful to introduce the *projections* of the ambient Riemann tensor onto $TS$: we can contract any of the indices of $R_{\mu\nu\rho\sigma}$ with either $n^\mu$ or $t_i^\mu$. For example,

$$R_{\boldsymbol{n}ijk} = n^\mu t_i^\nu t_j^\rho t_k^\sigma R_{\mu\nu\rho\sigma}\,, \tag{S1.8}$$

with obvious extension to other projections.

According to the fundamental theorem of surfaces, the knowledge of $h_{ij}$ and $K_{ij}$ completely determines the embedding $S$ up to isometries of $M_3$, provided they satisfy so-called compatibility relations. For the special case of two-manifolds embedded in three-manifolds, these relations are named after *Gauss*

$$R_{ijkl} = \mathcal{R}_{ijkl} - K_{[ij}K_{kl]}\,, \tag{S1.9}$$

and after *Codazzi-Mainardi*

$$R_{\boldsymbol{n}ijk} = \nabla_{[k}K_{j]i}\,. \tag{S1.10}$$

Embeddings of higher codimension must obey a further identity (the *Ricci relation*), which becomes trivial for the present case. In both Eq. (S1.9) and Eq. (S1.10) we made use of the projections of the Riemann tensor defined above.

The Gauss relation Eq. (S1.9) is often reported in its *contracted form*, which can be elegantly written as

$$\mathcal{R} = 2(K - G_{\boldsymbol{nn}})\,, \tag{S1.11}$$

where $\mathcal{R}$ is the Ricci scalar relative to $h_{ij}$, $K = \det K^i{}_j$ is the *Gaussian curvature* of $S$, and $G_{\boldsymbol{nn}}$ is the normal projection of the Einstein tensor

$$G_{\mu\nu} = R_{\mu\nu} - \frac{1}{2} g_{\mu\nu} R\,, \tag{S1.12}$$

where $R_{\mu\nu}$ is the Ricci tensor of $M_3$ and $R$ its scalar curvature.

Eq. (S1.11) becomes even simpler in the case of $M_3 = \mathbb{R}^3$, where the Einstein tensor vanishes and one is left with

$$\mathcal{R} = 2K\,, \tag{S1.13}$$

known also as *Gauss' theorema egregium.* Note that in this case - and in this case only - the intrinsic geometry of the embedding is determined entirely by the extrinsic curvature tensor.

The induced metric Eq. (S1.3) is all is necessary to compute the area element

$$\mathrm{d}A = \sqrt{\det h}\, d\sigma^1 d\sigma^2\,. \tag{S1.14}$$

From Eq. (S1.3) and Eq. (S1.7) we can define two coordinate-invariant extrinsic objects, namely the already introduced Gaussian curvature $K$ and the *mean curvature* $H$

$$K = \det K^i{}_j\,, \tag{S1.15a}$$

$$H = \frac{1}{2} h^{ij} K_{ij}\,. \tag{S1.15b}$$

### I.1. Shape equation

The starting point of our work is the bending energy Eq. (1) in the main text:

$$E_{\text{be}} = 2\kappa \int_S \mathrm{d}A H^2 \,, \tag{1}$$

of which we want to study its stationary points.

The derivation of the shape equation in $\mathbb{R}^3$ is a rather standard exercise, less so in arbitrary ambient manifolds: we report here the latter. Consider a small deformation $\delta r^\mu$ of $S$, which we can parametrize in terms of tangent and normal components as

$$\delta r^\mu = \Phi^i t_i^\mu + \Phi n^\mu \,, \tag{S1.16}$$

with arbitrary scalar functions $\Phi^i = \Phi^i(\sigma^j)$ and $\Phi = \Phi(\sigma^j)$ defined on $S$.

Plugging Eq. (S1.16) into Eq. (1) and expanding to first order terms in the deformation one obtains the differential equation that determines stationary surfaces. Reparametrization invariance of the bending energy guarantees that there cannot be bulk terms depending on tangent deformations $\Phi^i$. One is left with a single equation, the *shape equation* indeed, associated to normal deformations $\Phi$:

$$\Delta_S H + 2H\left(H^2 - K\right) + H R_{\boldsymbol{n}i\boldsymbol{n}}{}^i = 0 \,, \tag{S1.17}$$

where $\Delta_S = \nabla_i \nabla^i$ is the Laplace-Beltrami differential operator acting on the scalar quantity $H$. See e.g. [1] for a detailed derivation of Eq. (S1.17).

When $M_3 = \mathbb{R}^3$, this equation reduces to the Euclidean shape equation

$$\Delta_S H + 2H\left(H^2 - K\right) = 0 \,. \tag{S1.18}$$

*Minimal surfaces*, i.e. surfaces with $H = 0$ are always solutions of the shape equation Eq. (S1.17) in any ambient geometry.

The reason such surfaces are called "minimal" stems from the fact that having vanishing mean curvature is a necessary condition to be a local minimizer of the area functional

$$A = \int_S \mathrm{d}A \,, \tag{S1.19}$$

whose first variation under the deformation Eq. (S1.16) is

$$\delta^{(1)} A \propto \int_S \mathrm{d}A H \Phi \,, \tag{S1.20}$$

where the superscript "(1)" indicates a first-order variation (i.e. only linear terms in the deformation Eq. (S1.16) are kept). This expression holds for arbitrary $M_3$ and clearly vanishes whenever $H = 0$. See [1] for more details on these results and their generalizations to arbitrary dimensions.

### I.2. Stresses and the Darboux frame

For simplicity, in this Section we will focus mainly on the case of Euclidean ambient geometry, $M_3 = \mathbb{R}^3$.

If a surface is closed and smooth *up to third order*, then the Euclidean shape equation Eq. (S1.18) is the only differential condition a surface is subject to in order to minimize Eq. (1).

Nonetheless, when the variation Eq. (S1.16) is carried over a portion of the surface, it generates boundary terms. These boundary terms eventually determine the local force densities at any given point of the surface [2].

The smooth boundary $\partial S$ of a surface $S$ is a collection of closed curves. Each of these curves is naturally characterized by its Darboux frame, i.e. the curve's comoving frame which inherits its basis from the surface tangent and normal vectors.

On $\partial S$, the variation Eq. (S1.16) can be further decomposed as

$$\delta \boldsymbol{r} = \Phi_T \boldsymbol{T} + \Phi_N \boldsymbol{N} + \Phi \boldsymbol{n} \,, \tag{S1.21}$$

where $\boldsymbol{T} = T^i \boldsymbol{t}_i$ is the unit tangent vector of $\partial S$ and $\boldsymbol{N} = N^i \boldsymbol{t}_i$ is the unit tangent-normal Darboux vector. They are mutually orthogonal and satisfy $\boldsymbol{T} \cdot \boldsymbol{n} = \boldsymbol{N} \cdot \boldsymbol{n} = 0$.

Accordingly, the extrinsic curvature tensor Eq. (S1.7) can be decomposed into its Darboux components. We define

$$C_\parallel = K_{ij} T^i T^j \,, \tag{S1.22a}$$
$$C_\perp = K_{ij} N^i N^j \,, \tag{S1.22b}$$
$$\tau_g = -K_{ij} N^i T^j = -K_{ij} T^i N^j \,, \tag{S1.22c}$$

to be respectively the *normal curvature*, the *transverse curvature* and the *geodesic torsion* of the boundary $\partial S$. With this notation, we have $H = 1/2(C_\perp + C_\parallel)$ and $K = C_\perp C_\parallel$ on $\partial S$. Note that $C_\parallel$ and $C_\perp$ coincide with the surface principal curvature only when $\tau_g = 0$.

The complete first variation of Eq. (1) can be then written as

$$\delta^{(1)} E_{\text{be}} = -4\kappa \int_S \mathrm{d}A \, [\text{Eq. (S1.18)}] \, \Phi + \oint \mathrm{d}s B \,, \tag{S1.23}$$

where the bulk area term is given by the shape equation, while $s$ is the (Euclidean) arc-length of $\partial S$ and the boundary term $B$ is

$$\frac{B}{2\kappa} = \nabla_{\boldsymbol{N}} H \Phi + H^2 \Phi_N - H \nabla_{\boldsymbol{N}} \Phi \,, \tag{S1.24}$$

where $\nabla_{\boldsymbol{N}} = N^i \nabla_i = \boldsymbol{N} \cdot \boldsymbol{\nabla}$ is the surface-covariant directional derivative along the tangent-normal. Notice how in Eq. (S1.24) there is no Darboux tangent component $\Phi_T$, a consequence of the boundary reparametrization invariance.

The highest derivative of $\boldsymbol{r}$ appearing in Eq. (S1.24) is $\nabla_{\boldsymbol{N}} H$: since the mean curvature is a second-order quantity, this explains why third order smoothness is required in order to ignore boundary contributions to the stationarity condition.

Often Eq. (S1.24) is recast in terms of local force and torque densities. To see this, one must consider special rigid deformations of the form

$$\delta \boldsymbol{r} = \boldsymbol{a} + \boldsymbol{b} \times \boldsymbol{r} \,, \tag{S1.25}$$

for arbitrary constant vectors $\boldsymbol{a}$ and $\boldsymbol{b}$. This transformation corresponds to an (infinitesimal) translation along $\boldsymbol{a}$ followed by a rotation around the $\mathbb{R}^3$-coordinate origin with axis parallel to $\boldsymbol{b}$.

It is then easy to prove that Eq. (S1.24) becomes

$$B = \boldsymbol{a} \cdot \boldsymbol{\sigma} + \boldsymbol{b} \cdot (\boldsymbol{r} \times \boldsymbol{\sigma} + \boldsymbol{m}) \,, \tag{S1.26}$$

where $\boldsymbol{\sigma} = \boldsymbol{\sigma}_t + \boldsymbol{\sigma}_n$, with

$$\boldsymbol{\sigma}_t = \frac{\kappa}{2} \left( C_\parallel^2 - C_\perp^2 \right) \boldsymbol{N} \,, \tag{S1.27a}$$
$$\boldsymbol{\sigma}_n = 2\kappa \nabla_{\boldsymbol{N}} H \, \boldsymbol{n} \,, \tag{S1.27b}$$
$$\boldsymbol{m} = -2\kappa H \, \boldsymbol{T} \,, \tag{S1.27c}$$

being respectively the *tangential stress*, the *normal stress* and the *intrinsic torque* of the membrane at the boundary [2].

As explained in the main text, if the boundaryless surface $S$ is smooth up to second order but not to third order, then the only non-zero component of the stress is $\boldsymbol{\sigma}_n$, which quantifies the force density the membranes exerts at the contact lines along the the normal direction $\boldsymbol{n}$.

### I.3. The boundary conditions for adhesion

If part of the surface is adhering onto a substrate, then the fluctuation $\delta \boldsymbol{r}$ cannot be as arbitrary as in Eq. (S1.16), since even the free portion of the surface needs to follow the substrate at the detachment lines.

This requirement has an effect on the boundary conditions at contact lines [3]. Along this curve, it is extremely convenient to introduce *two* distinct Darboux frames, one relative to the free portion of the surface (labelled "(f)") and one relative to the bound part (labelled "(b)"), see [4] for more details.

The only possible deformation is along the substrate tangent-normal direction $\boldsymbol{N}_{(\text{b})}$, i.e. one has to replace Eq. (S1.21) with

$$\delta \boldsymbol{r} = \Phi_{(\text{b})} \boldsymbol{N}_{(\text{b})} \,. \tag{S1.28}$$

Note that while $\boldsymbol{N}_{(\mathrm{b})}$ is uniquely defined for a smooth surface (and coincides - up to orientation - with the Darboux tangent-normal $\boldsymbol{N}_{(\mathrm{f})}$ of the free portion of the surface), it is not the case for its tangent-normal derivatives. From Eq. (S1.28) we have that normal fluctuations are entirely suppressed, $\delta\boldsymbol{r}\cdot\boldsymbol{n}=0$: the substrate generates reaction forces that exactly balance the (eventual) tendency of the surface to detach or penetrate it. Using the Gauss-Weingarten relations we have

$$\nabla_{\boldsymbol{N}_{(\alpha)}}\Phi_n = \Phi_{(\mathrm{b})}\left(C_\perp^{(\alpha)} - C_\perp^{(\mathrm{b})}\right) , \tag{S1.29}$$

where $\alpha = \mathrm{f}, \mathrm{b}$. This derivative vanishes for the bound portion of the membrane, but does not vanish, in general, from the free portion (the transverse curvatures $C_\perp$ were defined in Eq. (S1.22b)).

Eq. (S1.29) has an effect on the boundary conditions since it enters Eq. (S1.24): a quick computation gives

$$B^{(\mathrm{f})} - B^{(\mathrm{b})} = \frac{1}{2}\kappa\left(C_\perp^{(\mathrm{f})} - C_\perp^{(\mathrm{b})}\right)^2 . \tag{S1.30}$$

If the energetic contribution of the adhering part of the surface is taken into account by a simple surface term $E_{\mathrm{ad}} = -wA_{\mathrm{ad}}$, then the difference Eq. (S1.30) must be compensated by $w$, leading to the famous adhesion contact condition

$$C_\perp^{(\mathrm{f})} = C_\perp^{(\mathrm{b})} - \frac{1}{R_w} , \tag{S1.31}$$

with $R_w = \sqrt{\kappa/2w}$. The sign convention is that $C_\perp^{(\mathrm{f})} > C_\perp^{(\mathrm{b})}$ would imply a penetration of the substrate by the free portion.

### I.4. Special conformal transformations

A special conformal transformation (SCT) is a coordinate transformation of the form

$$\boldsymbol{r} \to \frac{\boldsymbol{r} - \boldsymbol{c}|\boldsymbol{r}|^2}{1 - 2\boldsymbol{c}\cdot\boldsymbol{r} + |\boldsymbol{c}|^2|\boldsymbol{r}|^2} , \tag{S1.32}$$

for arbitrary constant vector $\boldsymbol{c}$. Together with rotations, translations and dilations (and compositions thereof), they are the only transformations that locally preserve angles. They form a group known as the *conformal group* which, in three dimensions, has dimension ten.

Note that the metric structure of Euclidean space changes under Eq. (S1.32), since these transformations are not isometries of $\mathbb{R}^3$ (this is immediately evident when Eq. (S1.32) act as an active transformation on an embedding: its graph gets heavily distorted).

If the map Eq. (S1.32) is acting on a surface embedded in $\mathbb{R}^3$, one has that the induced metric of the transformed surface is

$$h_{ij} \to \frac{1}{\Lambda^2}h_{ij} , \tag{S1.33}$$

with $\Lambda = 1 - 2\boldsymbol{c}\cdot\boldsymbol{r} + |\boldsymbol{c}|^2|\boldsymbol{r}|^2$. Since distances are distorted under Eq. (S1.32), curvatures are affected as well [5]

$$H \to \Lambda H + 2\lambda , \tag{S1.34a}$$
$$K \to \Lambda^2 K + 4\Lambda H\lambda + 4\lambda^2 , \tag{S1.34b}$$

with $\lambda = \left(\boldsymbol{c} - |\boldsymbol{c}|^2\boldsymbol{r}\right)\cdot\boldsymbol{n}$.

Note however that we can easily construct a combination of curvatures that *locally* does not change under a SCT: the expression

$$\mathrm{d}A\left(H^2 - K\right) , \tag{S1.35}$$

is a conformal invariant, i.e. it stays the same under Eq. (S1.32).

Because of the Gauss-Bonnet theorem and of the topological nature of Euler characteristic $\chi$ [6], also the bending energy Eq. (1) is invariant under conformal transformations. This can be easily seen if one rewrites it as

$$E_{\mathrm{be}} = 2\kappa\int_S \mathrm{d}A(H^2 - K + K) = 4\pi\kappa\chi + 2\kappa\int_S \mathrm{d}A(H^2 - K) . \tag{S1.36}$$

Note that this invariance is true as long as the surface is smooth up to second order and holds only globally, i.e. after the surface integral has been performed.

### I.5. Weyl transformations

A Weyl scaling is a *metric* transformation such that

$$g_{\mu\nu} \to e^{2\omega} g_{\mu\nu} \,, \tag{S1.37}$$

where $\omega(x^\mu)$ is an arbitrary smooth function. The line element transforms accordingly $ds^2 \to e^{2\omega} ds^2$. In the following we will again assume that $g_{\mu\nu}$ is arbitrary. Furthermore, we momentarily set the dimension of the ambient manifold to an arbitrary $d$ as some formulas will be useful for both $d = 2$ and $d = 3$. Much of what follows can be found e.g. in [7].

Under Eq. (S1.37), the ambient Christoffel symbols change as

$$\Gamma^\rho_{\mu\nu} \to \Gamma^\rho_{\mu\nu} + \delta^\rho_{(\mu}\partial_{\nu)}\omega - g_{\mu\nu} g^{\rho\alpha}\partial_\alpha\omega \,, \tag{S1.38}$$

so that the Riemann tensor transforms as

$$R_{\mu\nu\rho\sigma} \to e^{2\omega} \left(R_{\mu\nu\rho\sigma} + E_{\mu\nu\rho\sigma}\right) \,, \tag{S1.39}$$

where

$$E_{\mu\nu\rho\sigma} = g_{\mu[\sigma}\nabla_\nu\nabla_{\rho]}\omega - g_{\nu[\sigma}\nabla_\mu\nabla_{\rho]}\omega + g_{\nu[\sigma}\nabla_\mu\omega\,\nabla_{\rho]}\omega - g_{\mu[\sigma}\nabla_\nu\omega\,\nabla_{\rho]}\omega + g_{[\mu\sigma}g_{\nu]\rho}\nabla^\alpha\omega\,\nabla_\alpha\omega \,. \tag{S1.40}$$

Contracting the first and third index of this expression gives the transformation law for the Ricci tensor

$$R_{\mu\nu} \to R_{\mu\nu} - E_{\mu\nu} \,, \tag{S1.41}$$

which is scale invariant, with transformation tensor

$$E_{\mu\nu} = (d-2)\left(\nabla_\mu\nabla_\nu\omega - \nabla_\mu\omega\,\nabla_\nu\omega + g_{\mu\nu}\nabla_\lambda\omega\,\nabla^\lambda\omega\right) + g_{\mu\nu}\nabla^2\omega \,, \tag{S1.42}$$

and finally the Ricci scalar

$$R \to e^{-2\omega}\left(R - E\right) \,, \tag{S1.43}$$

with

$$E = 2\,(d-1)\,\nabla^2\omega + (d-2)\,(d-1)\,\nabla^\lambda\omega\,\nabla_\lambda\omega \,. \tag{S1.44}$$

Notice that for $d = 2$, the Ricci tensor and the Ricci scalar both transform with total derivatives.

With respect to surface embeddings, the Weyl rescaling induces changes on the adapted frame of the immersed surface, and consequently on its fundamental forms. The embedding functions $r^\mu$ are independent on the metric notions on the target space (as Eq. (S1.37) is not a coordinate transformation). Tangent vectors do not change as well, $t^\mu_i \to t^\mu_i$. The induced metric however, being defined via the scalar product in the ambient space, is affected, in the exact same manner as Eq. (S1.37)

$$h_{ij} \to e^{2\omega} h_{ij} \,, \tag{S1.45}$$

and analogously contravariant tangent vectors transform with the same weight $t_{i\mu} \to e^{2\omega} t_{i\mu}$. This implies that the area element also transforms as $\mathrm{d}A \to e^{2\omega}\mathrm{d}A$. The normalization of the normal vector imposes that it scales oppositely as the metric, $n^\mu \to e^{-\omega} n^\mu$. The extrinsic curvature tensor Eq. (S1.7) changes as

$$K_{ij} \to e^{\omega}\left(K_{ij} + h_{ij}\nabla_{\boldsymbol{n}}\omega\right) \,, \tag{S1.46}$$

with the covariant directional derivative $\nabla_{\boldsymbol{n}} = n^\mu \nabla_\mu$. From this we deduce the transformations

$$H \to e^{-\omega}\left(H + \nabla_{\boldsymbol{n}}\omega\right) \,, \tag{S1.47a}$$

$$K \to e^{-2\omega}\left(K + 2H\nabla_{\boldsymbol{n}}\omega + (\nabla_{\boldsymbol{n}}\omega)^2\right) \,. \tag{S1.47b}$$

Again, the combination Eq. (S1.35) is the only Weyl-invariant combination of $H$, $K$ and $\mathrm{d}A$. However, the bending energy $E_{\mathrm{be}}$, while being invariant under conformal transformations, is not a Weyl-invariant quantity [8].

The similarity between Eq. (S1.45) and Eq. (S1.33) are not coincidental: the effect on the induced metric of a SCT can be *undone* by a Weyl rescaling.

### I.6. Maximally symmetric spaces

Maximally symmetric spaces are manifolds that admit the maximum number of Killing vector fields for a given dimension. They have a remarkably simple Riemann tensor, namely

$$R_{\mu\nu\rho\sigma} = \pm\frac{\epsilon}{L^2}\left(g_{\mu\rho}g_{\nu\sigma} - g_{\mu\sigma}g_{\nu\rho}\right) , \tag{S1.48}$$

where $\epsilon$ is an arbitrary number and $L$ is the curvature scale of the space. Since the magnitude of $\epsilon$ can be adsorbed in a redefinition of $L$, it only matters if it is zero, positive or negative. Thus, in the following $\epsilon = 0, 1, -1$. The Ricci tensor and scalar are obtained by simple contractions

$$R_{\mu\nu} = \epsilon\frac{(d-1)}{L^2}g_{\mu\nu} , \quad \text{and} \quad R = \epsilon\frac{1}{L^2}d(d-1) . \tag{S1.49}$$

For three-dimensional manifolds, the only maximally symmetric spaces are: Euclidean space $\mathbb{R}^3$ ($\epsilon = 0$), the three-sphere $\mathbb{S}^3$ ($\epsilon = 1$) and the hyperbolic space $\mathbb{H}^3$ ($\epsilon = -1$).

A possible choice for the line element of these manifolds is

$$ds^2 = 4\frac{1}{\left(1 + \epsilon\frac{x^2+y^2+z^2}{L^2}\right)^2}ds^2_{\mathbb{R}^3} , \tag{S1.50}$$

with the three Cartesian coordinates $x, y, z$ and $ds^2_{\mathbb{R}^3} = dx^2 + dy^2 + dz^2$. The Ricci curvature of the above space is $R = \epsilon 6/L^2$. For $\epsilon = 1$ the metric Eq. (S1.50) reduces to the stereographic projection of $\mathbb{S}^3$ on $\mathbb{R}^3$. This projection is conformal, and some of the generators of $\mathbb{S}^3$ are realized indeed as the action of dilations and special conformal transformation.

When $\epsilon = -1$ in Eq. (S1.50), one obtains the *Poinaré ball* representation of $\mathbb{H}^3$. Note that in this case the space has a conformal boundary at $x^2 + y^2 + z^2 = L^2$. This metric in fact, characterizes *two* disjoint copies of $\mathbb{H}^3$, whose points satisfy either $x^2 + y^2 + z^2 > L^2$ or $x^2 + y^2 + z^2 < L^2$. Thus, it is more correct to say that Eq. (S1.50) describes the metric of the union $\mathbb{H}^3 \cup \mathbb{S}^2 \cup \mathbb{H}^3$, with the two-sphere $\mathbb{S}^2$ separating the two copies of $\mathbb{H}^3$.

For the hyperbolic case, there is an alternative representation known as the Poincaré half space model

$$ds^2 = \frac{L^2}{z^2}ds^2_{\mathbb{R}^3} , \tag{S1.51}$$

where the conformal boundary lies now at the plane $z = 0$. In this case, the geometry described by Eq. (S1.51) is $\mathbb{H}^3 \cup \mathbb{R}^2 \cup \mathbb{H}^3$.

Similarly to Eq. (S1.51), we will make use of the *Poincaré half-plane* model of $\mathbb{H}^2$

$$ds^2 = \frac{\ell^2}{z^2}ds^2_{\mathbb{R}^2} , \tag{S1.52}$$

with the conformal boundary now lying at the $z = 0$ *line*, and $\ell$ is the characteristic scale of the space. We will need this metric representation for the proof of Eq. (3) in the main text.

### I.7. Axisymmetric surfaces

Without loss of generality, an axisymmetric surface embedded in $\mathbb{R}^3$ can be parametrized in terms of two one-variable functions $r$ and $z$ as

$$\boldsymbol{r}(\sigma^1, \sigma^2) = \begin{pmatrix} r(\sigma^1)\cos\sigma^2 \\ r(\sigma^1)\sin\sigma^2 \\ z(\sigma^1) \end{pmatrix} , \tag{S1.53}$$

where $\sigma^2 \in [0, 2\pi]$ is the azimuthal angle. The pair $(r, z)$ draws a curve $\gamma$ in the half-plane which we call the *surface profile*. The full surface is thus a direct product $S = \mathbb{S}^1 \times \gamma$, with $\mathbb{S}^1$ the unit circle. A closed genus zero surface must necessarily have a surface profile that starts and ends at $r = 0$.

### I.7.1. Arc-length parametrization

It is very common (and often, very natural) to adopt an arc-length parametrization $\sigma^1 = \sigma^1(t)$ for the profile coordinate. This can be achieved by requiring

$$r'^2 + z'^2 = 1\,, \tag{S1.54}$$

where a prime $'$ indicates differentiation with respect to the arc-length parameter $t$. If this is the case, we can parametrize the tangent and normal vectors in terms of just one angle

$$r' = \cos\psi\,, \quad \text{and} \quad z' = \sin\psi\,, \tag{S1.55}$$

so that $\psi = \arctan z'/r'$ is the angle between the tangential meridian direction and the constant $z$ plane [9].

The induced metric Eq. (S1.3) and the curvature tensor Eq. (S1.7) are then

$$h_{ij} = \begin{pmatrix} r^2 & 0 \\ 0 & 1 \end{pmatrix}\,, \quad K_{ij} = -\begin{pmatrix} r\sin\psi & 0 \\ 0 & \psi' \end{pmatrix}\,, \tag{S1.56}$$

where $i = 2$ corresponds to the $t$ coordinate. The mean and Gaussian curvatures are then given by

$$H = -\frac{1}{2}\left(\psi' + \frac{\sin\psi}{r}\right) \qquad \text{and} \qquad K = \frac{\sin\psi}{r}\,\psi'\,. \tag{S1.57}$$

By our convention, $\psi = \pi/2$ corresponds to a vertical tangent vector pointing in the positive $z$ direction. Note the minus sign in the definition of $H$: a sphere of radius $\rho$, of parametrization $(r, z) = \rho(\sin t/\rho, \cos t/\rho)$ with $t \in [0, \pi]$ is such that $H = 1/R > 0$. The two principal curvatures are

$$C_\perp = -\psi'\,, \qquad \text{and} \qquad C_\parallel = -\frac{\sin\psi}{r}\,. \tag{S1.58}$$

We can now write down explicitly the bending functional $E_{\rm be}$ as

$$E_{\rm be} = \pi\kappa \int \mathrm{d}t \frac{(r\psi' + \sin\psi)^2}{r} = 4\pi\kappa\chi + \pi\kappa \int \mathrm{d}t \frac{(r\psi' - \sin\psi)^2}{r}\,, \tag{S1.59}$$

where in the second equality we used Eq. (S1.36).

Finally, it is instructive to write down the Laplace-Beltrami derivative of the mean curvature, since it is entering the shape equation Eq. (S1.18)

$$\Delta_S H = -\frac{1}{2}\psi''' - \frac{\cos\psi}{r}\psi'' + \frac{\sin\psi}{2r}\psi'^2 + \frac{\cos 2\psi}{2r^2}\psi' - \frac{\sin\psi\cos^2\psi}{2\mathbb{R}^3}\,. \tag{S1.60}$$

As it stands, this expression is rather complicated, and it is the main source of difficulties when solving the shape equation.

### I.7.2. Isothermal parametrization

For this reason, and because it will be essential for proving Eq. (3), we now introduce a second parametrization: isothermal coordinates. These are defined by a new parameter $\tau$ such that condition Eq. (S1.54) is changed to

$$\dot{r}^2 + \dot{z}^2 = r^2\,, \tag{S1.61}$$

where now the profile functions depend on $\tau$ rather than $t$, and we employ the overdot $\dot{}$ to emphasize this difference when taking derivatives. The relationship between the arc-length parameter $t$ and the isothermal parameter $\tau$ is given by

$$\mathrm{d}t = r\mathrm{d}\tau\,. \tag{S1.62}$$

Observe that while arc-length $t$ has the dimension of a length, $\tau$ is a pure number.

We then have that Eq. (S1.55) is replaced by

$$\dot{r} = r\cos\psi\,, \quad \text{and} \quad \dot{z} = r\sin\psi\,, \tag{S1.63}$$

where $\psi$ has exactly the same geometrical meaning as before.

The fundamental forms Eq. (S1.56) are now

$$h_{ij} = r^2 \begin{pmatrix} 1 & 0 \\ 0 & 1 \end{pmatrix} , \quad K_{ij} = -r \begin{pmatrix} \sin\psi & 0 \\ 0 & \dot{\psi} \end{pmatrix} . \tag{S1.64}$$

The fact that $h_{ij} = r^2 \delta_{ij}$ implies the property $\Delta_S \tau = 0$ of the parametrization, i.e. this coordinate choice is harmonic, hence the name "isothermal". We further have

$$H = -\frac{1}{2r}\left(\dot{\psi} + \sin\psi\right) \qquad \text{and} \qquad K = \frac{\dot{\psi}\sin\psi}{r^2} . \tag{S1.65}$$

and similarly

$$C_\perp = -\frac{\dot{\psi}}{r} , \qquad \text{and} \qquad C_\parallel = -\frac{\sin\psi}{r} . \tag{S1.66}$$

## II. PROOF OF EQ. 2

We have now all ingredients to prove Eq. (2) in the main text

$$E_{\text{be}} = \tilde{E}_{\text{be}} \pm \frac{2\kappa}{L^2}\tilde{A} . \tag{2}$$

Consider the behaviour under a Weyl transformation, Eq. (S1.37), of the integral density

$$\mathrm{d}A\left(H^2 - K + \frac{\mathcal{R}}{2}\right) . \tag{S2.1}$$

Given that $\mathrm{d}A(H^2 - K)$ is Weyl-invariant, the only term that changes is $\mathrm{d}A\,\mathcal{R}$, which, according to expression Eq. (S1.42) for $d = 2$, transforms with a total derivative. Thus we have the equality

$$\mathrm{d}A\left(H^2 - K + \frac{\mathcal{R}}{2}\right) = \mathrm{d}\tilde{A}\left(\tilde{H}^2 - \tilde{K} + \frac{\tilde{\mathcal{R}}}{2} + \tilde{\nabla}^2\omega\right) . \tag{S2.2}$$

where the tilde refers to quantities computed in the Weyl-transformed metric $\tilde{g}_{\mu\nu} = e^{2\omega} g_{\mu\nu}$. We can now make use of the contracted Gauss identity. Eq. (S1.11), obtaining

$$\mathrm{d}A\left(H^2 - G_{\boldsymbol{nn}}\right) = \mathrm{d}\tilde{A}\left(\tilde{H}^2 - \tilde{G}_{\boldsymbol{nn}} + \tilde{\nabla}^2\omega\right) . \tag{S2.3}$$

This identity holds for *any* initial ambient geometry $g_{\mu\nu}$. If we now restrict it to the case $M_3 = \mathbb{R}^3$, we have that the Einstein tensor $G_{\mu\nu}$ vanishes identically and integrating over a closed, smooth up to second order, surface we get rid of the total derivative $\tilde{\nabla}^2\omega$, leaving us with

$$E_{\text{be}} = \tilde{E}_{\text{be}} - 2\kappa \int_S \mathrm{d}A\tilde{G}_{\boldsymbol{nn}} , \tag{S2.4}$$

which holds for any *conformally flat* [10] three-manifold $\tilde{M}_3$. In this form, this result was first derived in [7].

If one picks as conformal factor $\omega$ the logarithms of the prefactors in metrics Eq. (S1.50) or Eq. (S1.51), then the transformed space is maximally symmetric, and thus, using Eq. (S1.49), we get

$$\tilde{G}_{\boldsymbol{nn}} = -\frac{\epsilon}{L^2} , \tag{S2.5}$$

which leads directly to Eq. (2) for $\epsilon = \pm 1$, completing the proof.

The main consequence of Eq. (2) is that minimal surfaces in $\tilde{M}_3$, i.e. surfaces with

$$\tilde{H} = 0 , \tag{S2.6}$$

are automatically stationary points of $E_{\text{be}}$, as follows from Eq. (S1.20). Note that this equation is inherently simpler than the shape equation Eq. (S1.18) (although, in general, with more terms than the analogous one in $\mathbb{R}^3$), since it involves only second derivatives of the embedding functions $r^\mu$. For more details see [7].

### II.1. A simple check

Although the area functional in Eq. (1) is always positive definite for any surface contained within a single copy of $\mathbb{H}^3$, it is not necessarily so if the surface crosses the conformal boundary and thus is contained in the extended space $\mathbb{H}^3 \cup \mathbb{S}^2 \cup \mathbb{H}^3$.

To illustrate this fact, consider a simple example: let us compute the right-hand side of Eq. (1) for a sphere of radius $\rho$ centred at the point $(0, 0, z_0)$, embedded in either $\mathbb{H}^3$ or $\mathbb{S}^3$ as described by the metric Eq. (S1.50).

We find for the bending energy

$$\tilde{E}_{\mathrm{be}} = 8\pi\kappa \frac{\left(\rho^2 - z_0^2 - \epsilon L^2\right)^2}{((\rho - z_0)^2 + \epsilon L^2)((\rho + z_0)^2 + \epsilon L^2)} , \tag{S2.7}$$

which correctly reduces to $\tilde{E}_{\mathrm{be}} = 8\pi\kappa$ for $\epsilon = 0$.

For the area we find

$$\tilde{A} = \frac{16\pi L^4 \rho^2 \epsilon}{((\rho - z_0)^2 + \epsilon L^2)((\rho + z_0)^2 + \epsilon L^2)} , \tag{S2.8}$$

which clearly is negative if $\epsilon = -1$ and $|L - z_0| < \rho < |L + z_0|$, i.e. if the sphere is embedded in hyperbolic space and crosses its conformal boundary.

Notice that for $\epsilon = 0$ the expression for the area *does not* reduce to the one of a sphere in $\mathbb{R}^3$, since the area functional is not Weyl-invariant. However, one recovers the common Euclidean formula by expanding Eq. (S2.8) for infinitesimal $\rho$ and $z_0 = 0$.

By plugging Eq. (S2.7) and Eq. (S2.8) into the right-hand side of Eq. (2) one readily obtains $8\pi\kappa$ for any $\epsilon$ and $L$, thus providing a good check on the correctness of our expression.

## III. PROOF OF EQ. 3

We can now prove Eq. (3) of the main text,

$$E_{\mathrm{be}} = 4\pi\kappa\chi + \pi\kappa\,\ell \int_\gamma \mathrm{d}\tau k^2 . \tag{3}$$

This follows directly from expression Eq. (S1.59), provided one uses the hyperbolic parameter $\tau$, defined in Eq. (S1.62), and introduces the quantity

$$k = \dot{\psi} - \sin\psi = r\left(C_\parallel - C_\perp\right) . \tag{S3.1}$$

What remains to show is that $k$ is indeed the *geodesic curvature* of a curve embedded in $\mathbb{H}^2$.

For a general two-manifold, the geodesic curvature is defined as

$$k = \mathtt{t}^i \mathtt{t}^j \nabla_i \mathtt{n}_j \tag{S3.2}$$

where $\mathtt{t}^i$ and $\mathtt{n}_i$ are the curve's tangent and normal two-vector fields.

Now consider the metric Eq. (S1.52) of the Poincaré half-plane representation of $\mathbb{H}^2$, which we write now as

$$ds^2 = \frac{\ell^2}{r^2}\left(dr^2 + dz^2\right) . \tag{S3.3}$$

A curve in this half-plane is parametrized by two functions $(r(\sigma), z(\sigma))$, where $\sigma$ is an arbitrary parametrization. The tangent and normal vectors to the curve are simply

$$\mathtt{t}^i = (\dot{r}, \dot{z}) , \tag{S3.4a}$$

$$\mathtt{n}^i = \frac{r}{\ell\sqrt{\dot{r}^2 + \dot{z}^2}}(\dot{z}, -\dot{r}) , \tag{S3.4b}$$

where a dot $\dot{}$ here denotes differentiation with respect to $\sigma$. Using the formula Eq. (S3.2) with the metric Eq. (S3.3) one finds

$$k = \frac{r}{\ell}\frac{\dot{r}\ddot{z} - \dot{z}\ddot{r}}{(\dot{r}^2 + \dot{z}^2)^{3/2}} - \frac{1}{\ell}\frac{\dot{z}}{(\dot{r}^2 + \dot{z}^2)^{1/2}} . \tag{S3.5}$$

Note that the first term in Eq. (S3.5) is the Euclidean expression for the geodesic curvature of a curve, multiplied by the conformal factor $r/\ell$.

If we now employ hyperbolic arc-length, i.e. a coordinate $\tau$ such that the tangent vector has unit norm,

$$\mathtt{t}^i\mathtt{t}_i = \ell^2\frac{\dot{r}^2+\dot{z}^2}{r^2} = 1\,, \tag{S3.6}$$

which can be achieved by requiring

$$\dot{r} = \frac{r}{\ell}\cos\psi\,,\quad \text{and}\quad \dot{z} = \frac{r}{\ell}\sin\psi\,, \tag{S3.7}$$

we see that Eq. (S3.5) corresponds exactly to the isothermal parametrization of an axisymmetric surface, Eq. (S1.63), provided $\ell = 1$ (i.e. $\ell$ is used as unit of length for the parameter $\tau$).

With Eq. (S3.7), the geodesic curvature Eq. (S3.5) reduces precisely to Eq. (S3.1), and this concludes our proof.

### III.1. Elastica equilibrium equation

The proven equivalence of Eq. (3) with the Euler elastica energy allows us to rewrite the shape equation, Eq. (S1.18), in a very simple form

$$\ddot{k} - k + \frac{k^3}{2} = 0\,. \tag{S3.8}$$

Quite remarkably, this expression is closed, i.e. it involves only $k$ and its second derivative. We emphasize how Eq. (S3.8) dramatically reduces the complexity of the of the Laplace-Beltrami operator with respect to standard Euclidean variables (see Eq. (S1.60) for comparison). The solutions of Eq. (S3.8) are Jacobi elliptic functions, and, in the next Section, they will allow us to derive Eq. (4) in the main text.

## IV. CONSTRUCTION OF THE HYPERBOLIC NECK SOLUTION, EQ. 4

In this Section we explain how Eq. (4),

$$\begin{pmatrix} r(\varphi) \\ z(\varphi) \end{pmatrix} = \frac{R\sinh\left(2b_p(0)\right)}{\cos\varphi + a_p(\varphi)\cosh b_p(\varphi)} \begin{pmatrix} \sqrt{p/(1-p)} \\ a_p(\varphi)\sinh b_p(\varphi) \end{pmatrix} \tag{4}$$

has been obtained.

There are two possible routes that lead to this result.

The first possibility is to make use of Eq. (2), namely of the fact that minimal surfaces in maximally symmetric spaces are solutions of the shape equation Eq. (S1.18). By writing explicitly the equation

$$\tilde{H} = 0\,, \tag{S4.1}$$

in terms of the profile functions, one sees that it can be solved analytically when the ambient manifold is $\mathbb{H}^3$ equipped with either the metric Eq. (S1.50) or Eq. (S1.51). The details of this type of derivation can be found in [11], where hyperbolic minimal surfaces ending on annular regions on the conformal boundary were constructed. One then has to apply a special conformal transformation of the type Eq. (S1.32) with $\boldsymbol{c}$ parallel to the rotational axis to obtain Eq. (4).

The alternative approach is to make use of Eq. (3) and of the solutions of the Euler elastica equation Eq. (S3.8) as described in detail in [1] (we remark that the solution was originally found by [12]).

We believe that it is more instructive to show here how to deal with the latter case.

The solutions of Eq. (S3.8) are of *five* kinds. Each kind is determined by whether the curvature is constant or not and by a single integration parameter. To see this, notice that if $\dot{k} = 0$ identically, then Eq. (S3.8) admits solutions with either $k = 0$ (*geodesics*) or $k^2 = 2$ (*constant geodesic curvature* curves, or CGC for short) [14]. Instead, if $\dot{k} \neq 0$ for some $\tau$, then we can multiply Eq. (S3.8) by $\dot{k}$ and integrate over $\tau$. One gets

$$\dot{k}^2 - k^2 + \frac{k^4}{4} = q^2 - 1\,, \tag{S4.2}$$

where $0 \leq q < \infty$ is an undetermined integration constant, whose value determines the type of the solution (see Table I). Solutions to Eq. (S4.2) can easily be expressed using the Jacobi $\mathrm{cn}(u,k)$ elliptic function.

| value of $q$ | $\mathbb{H}^2$ Elastica | $\mathbb{R}^3$ surface | minimal MSS surface |
|---|---|---|---|
| $q > 1$ | wavelike | the new solution Eq. (4) | $\mathbb{H}^3 \cup \mathbb{S}^2 \cup \mathbb{H}^3$ |
| $q = 1$ (1) | geodesics | spheres or planes | $\mathbb{H}^3 \cup \mathbb{S}^2 \cup \mathbb{H}^3$ |
| $q = 1$ (2) | asymptotically geodesic | catenoids & inverted catenoids | $\mathbb{R}^3$ |
| $0 < q < 1$ | orbitlike | – | $\mathbb{S}^3$ |
| $q = 0$ | CGC with $k^2 = 2$ | Clifford tori | $\mathbb{S}^3$ |

TABLE I. The five types of solutions of Eq. (S3.8). For each of them, we highlight how they can be interpreted as $\mathbb{H}^2$ elastica, axisymmetric Willmore surfaces and axisymmetric minimal surfaces embedded in maximally symmetric spaces (MSS), according to the diagram of Fig. 1a in the main text. The naming of the $\mathbb{H}^2$ curves follows the classification in [12]. CGC stands for constant geodesic curvature curve. The name "inverted catenoid" was first introduced in [13] and refers to SCT-transformed catenoids. Orbitlike curves correspon to self-intersecting tori in $\mathbb{R}^3$ (the profile, in general, is a covering of a circle with arbitrary homotopy class).

Once $k$ is found, we must integrate it further to find $\gamma$, i.e. the actual curve in the half-plane described by the profile functions $r$ and $z$. This can be achieved in an elegant manner if we make use of the fact that the vector field

$$\mathtt{v}_i = \frac{1}{2}k^2\mathtt{t}_i - \dot{k}\mathtt{n}_i\,, \tag{S4.3}$$

is Killing, i.e. it satisfies the Killing equation $\nabla_{(i}\mathtt{v}_{j)} = 0$ ($\mathtt{t}_i$ and $\mathtt{n}_i$ are the curve's unit tangent and normal vectors, introduced in Eq. (S3.4)). Since $\mathbb{H}^2$ is maximally symmetric, it turns out that $\mathtt{v}_i$ must be the restriction on $\gamma$ of a global Killing field.

In [1] it was proven that the integral curves of any Killing vector field in a maximally symmetric space is a CGC line. In $\mathbb{H}^2$ there are essentially three types of Killing vector fields: those who admit an integral geodesic, those that admit an integral horocycle and those who don't admit either. Ultimately, linking Eq. (S4.3) to any of those three types depends on the value of the constant $q$. This is so because the geodesic curvature $k_{\mathtt{v}}$ of an integral curve of Eq. (S4.3) at any point along $\gamma$ is given by

$$k_{\mathtt{v}} = \pm\frac{2k}{\sqrt{k^4+4\dot{k}^2}}\left(-1+\frac{4k^3\dot{k}}{k^4+4\dot{k}^2}\right) = k\frac{q^2-1+k^2\left(1-k\dot{k}\right)}{\left(q^2-1+k^2\right)^{3/2}}\,, \tag{S4.4}$$

which vanishes whenever $k = 0$. Points where the curvature vanishes are called *inflection points.* At inflection points the integral curve of $\mathtt{v}_i$ becomes a geodesic and intersects $\gamma$ orthogonally, since $\mathtt{v}_i \propto \mathtt{n}_i$.

Eq. (S4.2) tells us that inflection points exist if and only if $q \geq 1$. For $q = 1$ there is only one asymptotic inflection point, hence this solution was called in [12] *asymptoticlly geodesic.* For $q > 1$, $k$ has infinitely many inflection points: since each $\mathbb{H}^2$ Killing field has a unique integral geodesic, the curve must cross the *same* geodesic over and over and the solution oscillates (it "waves") around it, as shown in Fig. 1a of the main text. Conversely, for the case $0 \leq q < 1$ we have $k_{\mathtt{v}} \neq 0$ for every $\tau$, i.e. $\mathtt{v}_i$ does not admit any integral geodesic.

In more conventional Euclidean terms, an inflection point in $\mathbb{H}^2$ corresponds to an *umbilic point* on the axisymmetric surface, i.e. a point where the two principal curvatures coincide (see Eq. (S3.1): whenever $k = 0$ then $C_\perp = C_\parallel$). Since the contact lines between the neck and the plane/sphere *must* be umbilic in order to balance the in-plane stress, we can outright exclude solutions with $q < 1$.

We are then left with the $q \geq 1$ solutions to Eq. (S4.2), which we can write explicitly as

$$k(\tau) = \frac{2}{\sqrt{1-p}}\,\mathrm{cn}\left(\sqrt{\frac{1+p}{1-p}}\tau, \frac{1}{1+p}\right)\,, \tag{S4.5}$$

where $\mathrm{cn}(u,k)$ is a Jacobi elliptic function and we found more convenient to replace the parameter $q$ with

$$p = \frac{q-1}{q+1}\,, \tag{S4.6}$$

so that $p \in [0,1]$ for $q \geq 1$.

Now, Eq. (S4.3) must be the reduction on $\gamma$ of a $\mathbb{H}^2$ Killing field which admits an integral geodesic. Without loss of generality we can pick this Killing field to be $\{r, z\}$ - every other Killing field is linked to it by an $\mathbb{H}^2$ isometry. This field admits the half-line $z = 0$ as its integral geodesic, so that we can impose the relation

$$\mathtt{v} \propto (r, z)\,, \tag{S4.7}$$

where the proportionality constant is fixed by the boundary conditions. These can be computed by evaluating the expression at any inflection point [1]. Finally, the explicit form of the solution is now only one integration away:

$$2\frac{\dot{r}}{r} = (1-p)k\frac{\sqrt{p}k - (1-p)\dot{k}}{4p + (1-p)^2k^2}\,, \tag{S4.8a}$$

$$\frac{z}{r} = \frac{1-p}{2\sqrt{p}}k\,. \tag{S4.8b}$$

Using Eq. (S4.5), Eq. (S4.8) can be solved analytically. We find:

$$\begin{pmatrix} r(\tau) \\ z(\tau) \end{pmatrix} = \frac{e^{b_p(\tau)}}{a_p(\tau)} \begin{pmatrix} \sqrt{\frac{p}{1-p}} \\ -\cos\varphi(\tau) \end{pmatrix}\,, \tag{S4.9}$$

where

$$a_p(\tau) = \sqrt{\frac{1}{1-p} - \sin^2\varphi(\tau)}\,, \tag{S4.10a}$$

$$b_p(\tau) = \tilde{b}_p(\varphi = \pi/2) - \tilde{b}_p(\tau)\,, \tag{S4.10b}$$

with

$$\varphi(\tau) = \mathrm{amp}\left(\sqrt{\frac{1+p}{1-p}}\tau, \frac{1}{1+p}\right)\,, \tag{S4.11}$$

and

$$\tilde{b}_p(\tau) = \sqrt{\frac{p}{1-p^2}}\left(F\left(\varphi(\tau), \frac{1}{1+p}\right) - p\,\Pi\left(1-p; \varphi(\tau), \frac{1}{1+p}\right)\right)\,, \tag{S4.12}$$

where $\mathrm{amp}(u,k)$ is the Jacobi amplitude and $F(\phi,k)$ and $\Pi(n;\phi,k)$ are respectively incomplete elliptic integrals of the first and third kind (we use the same convention as *Mathematica* for the elliptic modulus $k$). At $\varphi = \pi/2$ we also have

$$\tilde{b}_p(\varphi = \pi/2) = b_p(0) = \sqrt{\frac{p}{1-p^2}}\left(K\left(\frac{1}{1+p}\right) - p\,\Pi\left(1-p; \frac{1}{1+p}\right)\right)\,, \tag{S4.13}$$

where now the elliptic integrals are complete and depend only on the elliptic moduli. Note that the function $b$ in Eq. (S4.10) has a more compact integral representation, which is reported in the main text below Eq. (4).

Since both the geodesic curvature, Eq. (S4.5), and the profile functions, Eq. (S4.9), depend on $\tau$ through $\varphi(\tau)$, we can simply employ $\varphi$ as independent variable.

Eq. (S4.9) describes a curve that oscillates around the vertical geodesic $z = 0$. It is easy to verify that

$$\begin{pmatrix} r(\varphi + n\pi) \\ z(\varphi + n\pi) \end{pmatrix} = e^{-2b_p(0)n} \begin{pmatrix} r(\varphi) \\ z(\varphi) \end{pmatrix}\,, \tag{S4.14}$$

for any $\varphi$ and $n \in \mathbb{N}$. This relation shows how the curve exhibits affine self-similarity, where the shape of the curve between two consecutive inflection points is repeated identically, up to scale transformations. Although the period of an oscillation is $2\pi$ (in the $\varphi$ variable), the self-similar pattern repeats every half-period up to reflections around the geodesic. We can thereofre focus to $\varphi \in [-\pi/2, \pi/2]$. The two inflection points at $\varphi = \pm\pi/2$ have coordinates

$$\begin{pmatrix} r(\pi/2) \\ z(\pi/2) \end{pmatrix} = \begin{pmatrix} 1 \\ 0 \end{pmatrix} \quad \text{and} \quad \begin{pmatrix} r(-\pi/2) \\ z(-\pi/2) \end{pmatrix} = \begin{pmatrix} e^{2b_p(0)} \\ 0 \end{pmatrix}\,. \tag{S4.15}$$

Now we can use the isometries of $\mathbb{H}^2$ to map this solution to the neck solution described in the main text. The isometry group of Lobachevsky space is isomorphic to $SO(1,1)$ and has three generators; not surprisingly, this group is also isomorphic to the centralizer of a rotation within the conformal group in three dimensions. The three generators can be chosen to be a translation along the $z$ axis, a dilation and a SCT, see Eq. (S1.32), with $\boldsymbol{c} = (0,0,c)$.

Since, by construction, the geodesic curvature is always invariant under isometries [15], we have that any property of $k$ will be preserved under isometric transformations. In particular, we already showed how inflection points with $k = 0$ correspond to umbilic points of the original surface. We thus have that *umbilicity is preserved under special conformal transformations*. Therefore, we can map the two points Eq. (S4.15) to any two points in the half-plane, and we are guaranteed that the curve profile outlined for $-\pi/2 \leq \varphi \leq \pi/2$ will smoothly connect two umbilic points.

While the effect of translations and scalings is trivial, SCTs require a bit more attention. Explicitly, the only SCT compatible with the isometries of the Poincaré model of $\mathbb{H}^2$ is

$$\begin{pmatrix} r \\ z \end{pmatrix} \to \frac{1}{1+2cz+c^2(r^2+z^2)} \begin{pmatrix} r \\ z+c(r^2+z^2) \end{pmatrix} , \tag{S4.16}$$

for an arbitrary constant $c$. This transformation maps the straight line $z = 0$ to the half-circle of radius $\frac{1}{2c}$ centered at $(0, \frac{1}{2c})$. This half-circle will be the locus of the two contact points (see Fig. 2a). For $c = 1/2$, this solution is mapped, up to scalings and translations, to a solution that joins a sphere at $\varphi = -\pi/2$ to a plane at $\varphi = \pi/2$. Fixing the sphere radius to $R$ and the location of the plane at $z = 0$ completely determines the isometric transformation that leads to Eq. (4).

### IV.1. Analytic expression of geometric quantities

From the analytic solution Eq. (4) we can derive expressions for all the relevant geometric quantities of the neck discussed in the main text.

The radial coordinates of the neck-plane and neck-sphere contact lines are respectively

$$\begin{pmatrix} r(\pi/2) \\ z(\pi/2) \end{pmatrix} = R \begin{pmatrix} \sinh 2b_p(0) \\ 0 \end{pmatrix} , \tag{S4.17a}$$

$$\begin{pmatrix} r(-\pi/2) \\ z(-\pi/2) \end{pmatrix} = R \begin{pmatrix} \tanh 2b_p(0) \\ \sinh 2b_p(0) \tanh 2b_p(0) \end{pmatrix} , \tag{S4.17b}$$

while the tangent angles are

$$\tan\psi(\pi/2) = 0 , \tag{S4.18a}$$

$$\tan\psi(-\pi/2) = \sinh 2b_p(0) . \tag{S4.18b}$$

Since the radius of the sphere is $R$, from Eq. (S4.17) and Eq. (S4.18) we get Eq. (6) of the main text for the sphere-plane distance

$$d = R\cosh 2b_p(0) . \tag{6}$$

Notice that the maximum distance $d^*$ can be found by taking the derivative with respect to $p$ of the distance,

$$\frac{d}{dp}d = \sqrt{\frac{d^2-R^2}{p(1-p)}} \left( 2E\left(\frac{1}{1+p}\right) - K\left(\frac{1}{1+p}\right)\right) , \tag{S4.19}$$

and setting it equal to zero. Here, $E(k)$ and $K(k)$ are the complete integrals of the first and second kind. The equation $2E(k) = K(k)$ cannot be solved analytically, but has a single solution $k^* \simeq 0.826$ which leads to the value $p^* \simeq 0.210$ mentioned in the main text.

Furthermore, from Eq. (S4.18) we get the *wrapping degree* $\alpha$ of the particle, i.e. the fraction of its area that is covered by the membrane

$$\alpha = \frac{1+\operatorname{sech} 2b_p(0)}{2} = \frac{1}{2}\left(1+\frac{R}{d}\right) . \tag{S4.20}$$

The latter equality gives a notably simple geometric relation between wrapping fraction and distance.

The mean curvature has a slightly more complicated expression

$$H = -\frac{1}{Ra_p(\varphi)\sinh\left(2b_p(0)\right)} \left( \frac{\sqrt{p}}{1-p}\cos\varphi\cosh b_p(\varphi) + \dot{\varphi}\sin\varphi\sinh b_p(\varphi)\right) , \tag{S4.21}$$

where, from Eq. (S4.11), $\dot{\varphi} = \frac{d\varphi}{d\tau} = \sqrt{\frac{p+\cos^2\varphi}{1-p}}$. Eq. (S4.21) satisfies $H = 0$ for $\varphi = \pi/2$ and $H = 1/R$ for $\varphi = -\pi/2$. Similarly, the tangent-normal derivative of the mean curvature, which enters the expression for the normal stress Eq. (S1.27b), is

$$\nabla_{\boldsymbol{N}} H = \frac{\cos\varphi + a_p(\varphi)\cosh b_p(\varphi)}{R^2 a_p(\varphi)\sqrt{p(1-p)}\sinh^2\left(2b_p(0)\right)} \left(\cos^3\varphi\sinh b_p(\varphi) - \dot{\varphi}\sqrt{p}\sin\varphi\cosh b_p(\varphi)\right) , \tag{S4.22}$$

which when evaluated at the contact lines gives

$$\nabla_{\boldsymbol{N}} H|_{\varphi=-\pi/2} = \frac{1}{R^2 \tanh^2(2b_p(0))} \frac{\sqrt{p}}{1-p} \qquad \text{and} \qquad \nabla_{\boldsymbol{N}} H|_{\varphi=-\pi/2} = \frac{1}{R^2 \sinh^2(2b_p(0))} \frac{\sqrt{p}}{1-p} \,. \tag{S4.23}$$

Note that the direction of $\boldsymbol{N}$ is parallel to $\partial_\tau$ along the neck-plane contact line, while it is antiparallel to it along the neck-sphere contact line.

The individual principal curvatures can be obtained by combining Eq. (S4.21) with the difference

$$C_{\parallel} - C_{\perp} = \frac{2\cos\varphi}{R\sqrt{p}\sinh(2b_p(0))} \left(\cos\varphi + a_p(\varphi)\cosh b_p(\varphi)\right) \,. \tag{S4.24}$$

The bending energy can also be computed exactly, it is sufficient to plug Eq. (S4.5) in Eq. (3) with the appropriate boundary conditions given by Eq. (S4.11). One finds the expression given by Eq. (7) in the main text, or, in terms of complete elliptic functions

$$e(p) = \frac{1}{\sqrt{1-p^2}} \left( (1+p)E\left(\frac{1}{1+p}\right) - pK\left(\frac{1}{1+p}\right) \right) \,. \tag{S4.25}$$

Rather interestingly, the energy is minimized at the same $p$ value at which $d$ is maximized. This can be easily checked by computing $\frac{de(p)}{dp}$.

Finally, the radius of the neck $R_{\mathrm{ne}}$ is found by imposing

$$\frac{1}{r(\varphi)} \frac{d}{d\varphi} r(\varphi) = \cos\psi(\varphi) = \frac{(a_p(\varphi) + \cos\varphi\cosh b_p(\varphi))\sin\varphi - \frac{\sqrt{p}}{\dot{\varphi}(1-p)}\cos^2\varphi\sinh b_p(\varphi)}{a_p(\varphi)\left(\cos\varphi + a_p(\varphi)\cosh b_p(\varphi)\right)} = 0 \,, \tag{S4.26}$$

which, although not solvable analytically, can be easily solved numerically for $\varphi$.

### IV.2. The adhesion equation

In the case of non-zero adhesion potential $w$, we have to modify the boundary condition at the neck-sphere contact line according to Eq. (S1.31). Since the sphere is a totally umbilic surface, we have that $C_{\parallel}^{(\mathrm{b})} = C_{\perp}^{(\mathrm{b})} = 1/R$. Therefore the adhesion matching conditions become

$$C_{\perp}^{(\mathrm{f})} = \frac{1}{R} - \frac{1}{R_w} \,, \tag{S4.27a}$$

$$C_{\parallel}^{(\mathrm{f})} = \frac{1}{R} \,. \tag{S4.27b}$$

These two equations serve to fix *two* parameters: the value of $\varphi = \bar{\varphi} \geq -\pi/2$ at which matching of the transverse curvature is possible, and the overall scaling of the solution so that the connecting sphere has effectively radius equal to $R$. As they stand, both these expressions depend non-trivially on these quantities; notice however that we can divide the first equation by the second and obtain a scale-independent relation

$$\frac{C_{\perp}^{(\mathrm{f})}}{C_{\parallel}^{(\mathrm{f})}} = 1 - \frac{R}{R_w} \,, \tag{S4.28}$$

which allows us to determine first $\bar{\varphi}$ for any given value of the dimensionless ratio $\frac{R}{R_w}$ (and for a fixed value of $p$), and only then fix the scale factor so that Eq. (S4.27b) is satisfied. We can write this equation explicitly by means of Eq. (S4.21) and Eq. (S4.24):

$$1 - \frac{C_{\perp}^{(\mathrm{f})}}{C_{\parallel}^{(\mathrm{f})}} = \frac{2a_p(\varphi)\cos^2\varphi\left(\cos\varphi + a_p(\varphi)\cosh b_p(\varphi)\right)}{\cos^2\varphi\left(a_p(\varphi) + \cos\varphi\cosh b_p(\varphi)\right) - \sqrt{p}\dot{\varphi}\sin\varphi\sinh b_p(\varphi)} = \frac{R}{R_w} \,, \tag{S4.29}$$

at $\varphi = \bar{\varphi}$.

Eq. (S4.29) can be easily solved numerically, allowing us to derive the results shown in Fig. 3. Notice that if $R/R_w = 0$, it admits as only solution $\bar{\varphi} = \pm\pi/2$.

---

[1] P. Fonda, V. Jejjala, and A. Veliz-Osorio, Annals of Physics **385**, 358 (2017), arXiv:1611.03462.

[2] R. Capovilla and J. Guven, Journal of Physics A: Mathematical and General **35**, 302 (2002), arXiv:0203148 [cond-mat].
[3] U. Seifert and R. Lipowsky, Physical Review A (1990), 10.1103/PhysRevA.42.4768.
[4] M. Deserno, M. M. Müller, and J. Guven, Physical Review E **76**, 011605 (2007), arXiv:0703019 [cond-mat].
[5] E. Abbena, S. Salamon, and A. Gray, *Modern differential geometry of curves and surfaces with Mathematica* (Chapman and Hall/CRC, 2017).
[6] This is not necessarily true in the case of a surface with boundaries.
[7] P. Fonda, D. Seminara, and E. Tonni, Journal of High Energy Physics **2015**, 1 (2015).
[8] The reason for this is that the Gauss-Bonnet theorem holds for the integral of the surface's Ricci scalar, and *not* for the integral of the Gaussian curvature. This subtle difference is lost when the ambient space is $\mathbb{R}^3$ because of the Theorema Egregium.
[9] Technically, the inverse map from $(z', r')$ to $\psi$ should carefully take into account the sign of both components of the tangent vector. A way to do so is to define $\psi = \text{atan2}(r', z')$ with the customary $C$ function atan2.
[10] A manifold is conformally flat if its metric can be written as $\Lambda^2\delta_{\mu\nu}$, i.e. if a Weyl scaling can map it to Euclidean space.
[11] P. Fonda, L. Giomi, A. Salvio, and E. Tonni, Journal of High Energy Physics **2015**, 5 (2015).
[12] J. Langer and D. A. Singer, Journal of Differential Geometry (1984), 10.4310/jdg/1214438990.
[13] P. Castro-Villarreal and J. Guven, Physical Review E **76**, 011922 (2007).
[14] The sign of the geodesic curvature is not really relevant since it reflects the sign ambiguity in the definition of the normal vectors.
[15] In Euclidean space this is trivially true: the curvature of a curve is independent on its location or orientation in space.
